# Supplementary material for: Nonlinear dynamic analysis of an epidemiological model for COVID-19 including public behavior and government action
Source: arXiv:2006.09530 source file (2020-10-14)
Supplement: Supplementary file 1 [file appendix.tex]

% appendix.tex

\section*{Appendix}
\paragraph{Proof}
The equation of $I_{c0}^*$ shows that a solution is the intersection of the following graphs
\beq Z(X)=X,~~~Y(X)=\frac{I_0}{R_0-1}\left[1-\frac{1+N}{(1-mX)^{\kappa}}\right]\eeq
with $m=\frac{d\gamma}{\lambda}$ and $N=\frac{\beta_1\sigma}{\beta_2(\gamma+\mu)}$
The intersection point in the interval $[0,1]$ will exist if
\beq R_0-1>\frac{\beta_1\sigma}{\beta_2(\gamma+\mu)}\eeq
\begin{figure}[!ht]
    \begin{center}
        \includegraphics[scale=0.5]{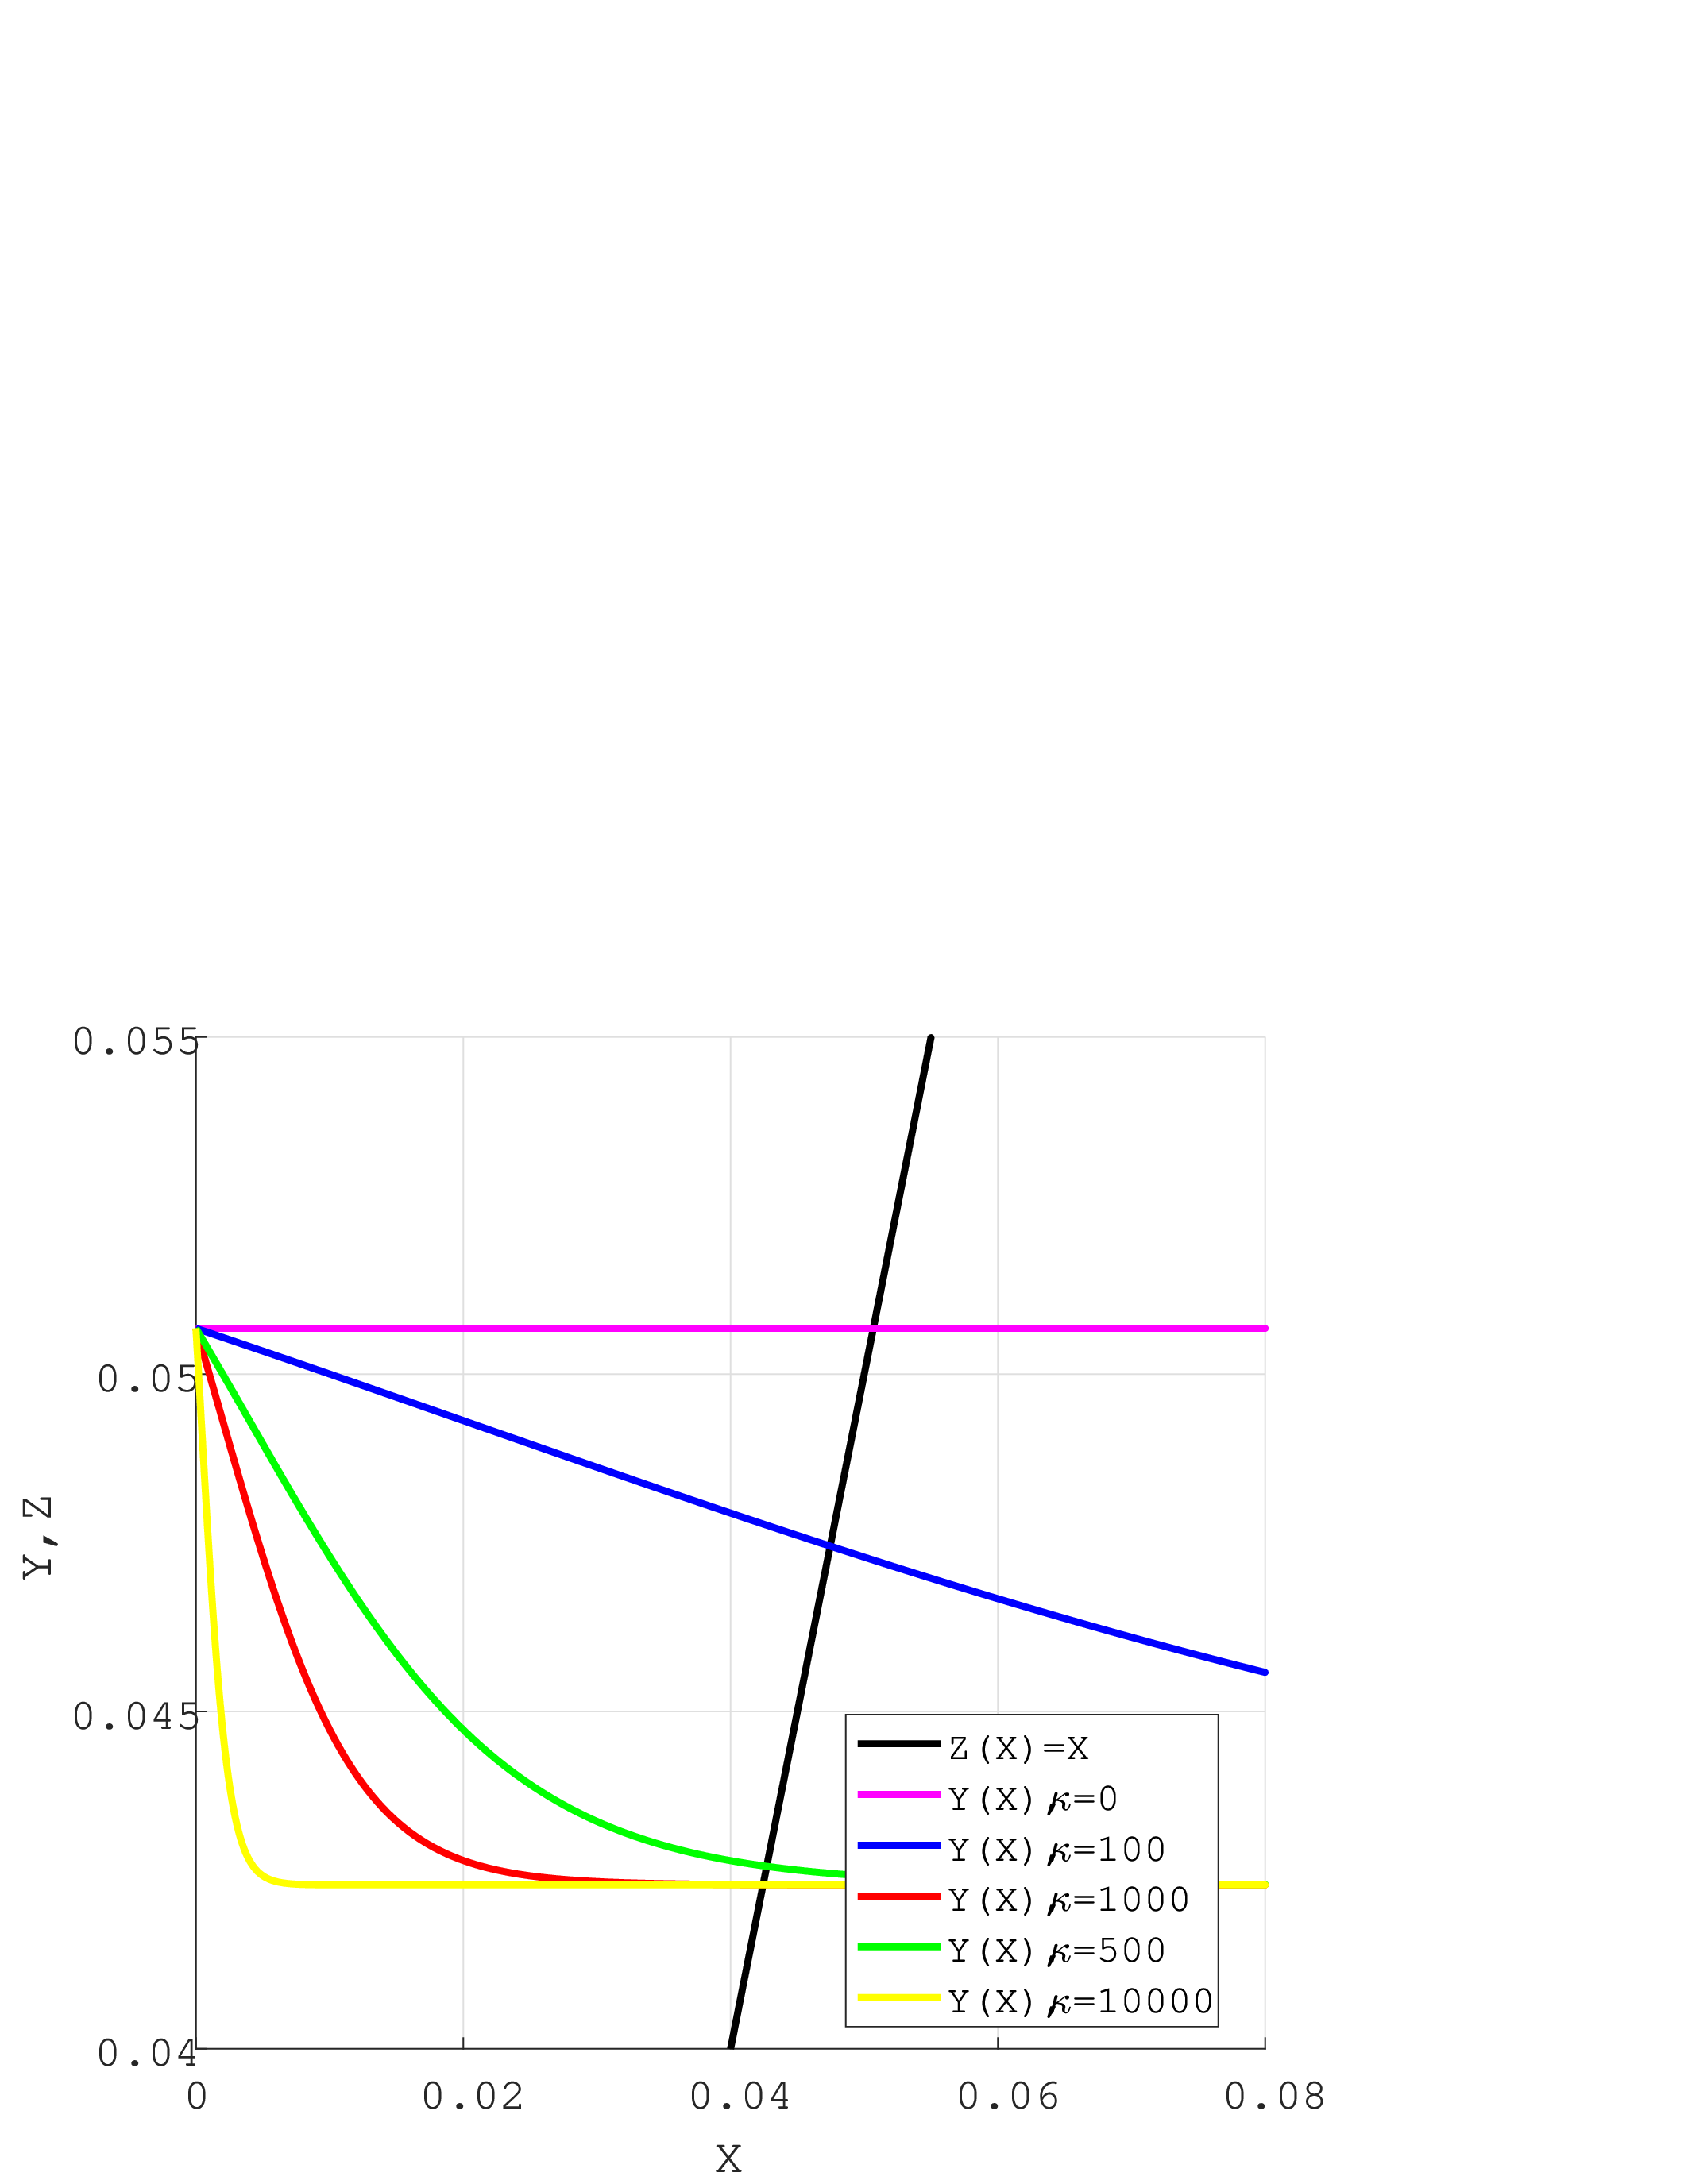}
\caption{}
\label{fig8}\end{center}
   \end{figure}
